# Supplementary material for: Approximation of optimization problems with constraints through kernel Sum-Of-Squares
Source: arXiv:2301.06339 source file (2024-02-21)
Supplement: Supplementary file 1 [file appendix.tex]

\section{Extra results}

	\subsection{Closedness of curl-free and group-invariant}

	\begin{proposition}\label{lem:group_kernel}
		Let $(\hh, \scalh{\cdot}{\cdot})$ be a $R^P$-valued vRKHS with kernel $K$. Set $\hh_G:=\{\b f \in \hh\,|\, \forall g\in G,\, \b f\circ g=\b f\}$, then $(\hh_G, \scalh{\cdot}{\cdot})$ is a vRKHS. Assume that (i) there exists\todo{which properties for $\psi$?} $\psi:G\rightarrow G$ such that $ K(g\cdot x, y)=K(x, \psi(g)\cdot y)$ for all $g\in G$ and $x,y\in \X$, (ii) $G$ has a normalized Haar measure $\mu$, (iii) the kernel $K_G(x,y):=\iint_{G\times G} K(g\cdot x,g'\cdot y) \d \mu(g) \d \mu(g')$ has finite values for all $x,y\in \X$. Then $K_G$ is the reproducing kernel of $\hh_G$. 
		
		Moreover if the function $x\mapsto K(g \cdot x,y )\b p$ belongs to $\hh$ for all $y\in \X$, $g\in G$ and $\b p\in\R^P$, and, setting $\hh_0:=\Sp(\{K(\cdot,x)\b p\}_{x\in\X,\b p\in\R^P})\subset \hh$, for every $g\in G$, the operator $T_g:f\in\hh_0\mapsto f\circ g\in\hh_0$ is bounded for $\norh{\cdot}$, then, for all $g\in G$ and $\b f \in \hh$, $f\circ g\in\hh$.
	\end{proposition}
	\begin{proof}
		Applying \Cref{lem:closed_subspaces} to $\hh_G$, which is a special case of $E_G\cap \hh$, gives that $(\hh_G, \scalh{\cdot}{\cdot})$ is a vRKHS since it is a closed subspace of the vRKHS $\hh$.
		\todo[inline]{show that: For any $y\in\X$ and $\b p\in\R^P$, $K_G(\cdot,y)\b p\in \hh$ and that one can exchange integral and inner product}
		Fix any $\b f\in\hh_G$, $y\in\X$ and $\b p\in\R^P$,%
		\begin{align*}
		\scalh{\b f}{K_G(\cdot,y)\b p}&=\iint_{G\times G} \scalh{\b f}{K(\cdot,\psi(g)\cdot g'\cdot y)\b p} \d \mu(g) \d \mu(g')\\
		&=\iint_{G\times G} \b p^\top \b f(\psi(g)\cdot g'\cdot y) \d \mu(g) \d \mu(g')\stackrel{\b f\in\hh_G}{=}\b p^\top \b f(y).
		\end{align*}
		Consequently $K_G$ is the reproducing kernel of $(\hh_G, \scalh{\cdot}{\cdot})$. Moreover since $\hh_0$ is dense in $\hh$, for any $\b f\in\hh$ we can find a sequence $(\b f_n)_{n\in N}\in (\hh_0)^\N$ converging to $\b f$. Since $(\|\b f_n\|)_{n\in N}$ is then bounded and $T_g$ is bounded over $\hh_0$, the sequence $(\|\b f_n\circ g\|)_{n\in N}$ is also bounded in $\hh$. As $K_G(\cdot,g\cdot x)\in\hh$, by the reproducing property and the weak convergence of $(\b f_n)_{n\in N}$, we have that $\b p^\top\b f_n(g\cdot x)=\scalh{\b f_n}{K_G(\cdot,g\cdot x)\b p}\rightarrow \b p^\top\b f(g\cdot x)$. As $(\b f_n\circ g)_{n\in N}$ is bounded in $\hh$, it has weakly converging subsequence to some $\b h\in \hh$ which is necessarily equal pointwise to $\b f\circ g$. Hence $\b f\circ g\in \hh$.
		
	\end{proof}
	
	Note: we chose to leverage classical tools from set-valued analysis to tackle the problem of the existence of regular solutions satisfying the constraints. An alternative would have been to use inverse functions theorems if we had an explicit expression $\b F(x):=\{y \,|\, g_i(x,y)\le 0, \, \forall i\in [I] \}$. However this would have required a detailed analysis of the regularity of the functions $g_i$ and would have left open the problem of the lack of regularity of the constraints set when taking intersections for $I>1$.

	\subsection{Existence of measurable solution}
	We have the extension of CITE ciliberto Lemma A.1 p38
	
	\begin{lemma}[Existence of a minimizer for the expected risk] Let $\X\times\Y$ be a complete measure space\todo{check assumption on $\Y$, Polish?} and $\Z$ be a complete separable metric space. Let $\Delta: \Z \times \Y \rightarrow \R$\todo{finite values seems mandatory} be a continuous function and $F:\X\leadsto \Z$ be a measure set-valued map with closed non-empty images. Then, the expected risk $\E(f)=\int_{\X\times \Y} \Delta(f(x), y) d \rho(x,y)$ admits a measurable minimizer $f^*: \X \rightarrow \Z$ such that
		$$
		f^*(x) \in \underset{z \in F(x)}{\operatorname{argmin}} \int_{\Y} \Delta(z, y) d \rho(y \mid x)
		$$
		almost everywhere on $D_{\rho \mid \X} .$ Moreover, the function $m: \X \rightarrow \R$ such that
		$$
		m(x)=\inf_{z \in F(x)}  r(x, z), \quad \text { with } \quad r(x, z)=\left\{\begin{array}{cc}
		\int_{\Y} \Delta(z, y) d \rho(y \mid x) & \text { if } x \in D_{\rho \mid \X} \\
		0 & \text { otherwise }
		\end{array}\right.
		$$
		for any $x \in \X$, is measurable.
	\end{lemma}
	\begin{proof}
		Since $\Delta$ is continuous and $\rho(y \mid x)$ is a regular conditional distribution (Dudley 2002), then $r$ is a Carathéodory function (see Definition $4.50$ (pp. 153) in Aliprantis and Border, 2006), namely continuous in $z$ for each $x \in \X$ and measurable in $x$ for each $z \in F(x)$. Thus, by \citet[][Theorem 8.2.11, p316]{aubin1990sva}, we have that $m$ is measurable and, by \citet[][Theorem 8.2.10, p316]{aubin1990sva}, that there exists a measurable $f^*: \X \rightarrow \Z$ such that $f(x)\in F(x)$ and $r\left(x, f^*(x)\right)=m(x)$ for almost every $x \in \X$. Moreover, by definition of $m$, given any measurable $f: \X \rightarrow \Z$, we have $m(x) \leq r(x, f(x)) .$ Therefore
		$$
		\E\left(f^*\right)=\int_{\X} r\left(x, f^*(x)\right) d \rho_{\X}(x)=\int_{\X} m(x) d \rho_{\X}(x) \leq \int_{\X} r(x, f(x)) d \rho_{\X}(x)=\E(f)
		$$
		We conclude $\E\left(f^*\right) \leq \inf_{f: \X \rightarrow \Z, f(x)\in F(x) \text{ a.e.\ } x} \E(f)$ and, since $f^*$ is measurable and satisfies the constraints, $\E\left(f^*\right)=\min_{f: \X \rightarrow \Z, f(x)\in F(x) \text{ a.e.\ } x} \E(f)$ and $f^*$ is a global minimizer.
	\end{proof} 

	\subsection{Remainders of looking into Lang 1995}

	Hence we can find an atlas $\{(G_\alpha,\gamma_\alpha)\}_{\alpha\in \A}$, where $\A$ is an arbitrary index set, that is subordinated to $(\BB(x,\delta_x))_{x\in\X}$ (i.e.\ for each $G_\alpha$ there exists a $\BB(x,\delta_x)$ containing it) and such that $\gamma_\alpha G_\alpha = \Ecal$. Since $\X$ is a metric space, it is paracompact \citep[][Corollary 1]{stone1948paracompact}, so we can find an open refinement $\left\{U_{x}\right\}_{x\in\X}$ of the covering $\left\{G_{\alpha}\right\}$ (i.e.\ each $U_{x}$ is an open set contained in some $G_{\alpha(i)}$ and $\X=\bigcup_{x\in\X}U_{x}$) which is locally finite (i.e.\ for every $x_0\in\X$, there exists a neighborhood of $x_0$ which intersects only a finite number of $U_i$). Let $\varphi_{x}$ be the restriction of $\gamma_{\alpha(i)}$ to $U_{x}$. Again by paracompactness of $\X$, without having change to the index set \citep[][Proposition 3.1, p.\ 31]{lang1995diff}, we can find locally finite open refinements  $\left\{V_{x}\right\}_{x\in\X}$, and then $\left\{W_{x}\right\}_{x\in\X}$, applying \citep[][Proposition 3.3, p.\ 31]{lang1995diff}, of $\left\{U_{x}\right\}_{x\in\X}$, such that
	$$
	\bar{W}_{x} \subset V_{x} \subset \bar{V}_{x} \subset U_{x}
	$$
	the bar denoting closure in $\X$. Each $\bar{V}_{x}$ being closed in $\X$, we consequently have that $\varphi_{x} \bar{V}_{x}$ is closed in $\Ecal$, and so is $\varphi_{x} \bar{W}_{x}$. Using \citet[][Theorem 3.7, p.\ 36]{lang1995diff},\todo{to detail} and transporting functions on $\Ecal$ to functions on $\X$ by means of the $\varphi_{x}$, we can find for each $i$ a function $\psi_{x} \in C^m(\X,[0,1])$ with is 1 on $\bar{W}_{x}$ and 0 on $\X\backslash V_{x}$. By transitivity, $\left\{V_{x}\right\}_{x\in\X}$ is a refinement of $\left\{\BB(x,\delta_x)\right\}_{x\in\X}$ so, for each $i\in \Ical$, we can fix $x_i\in\X$ such that $V_{x}\subset \BB(x_i,\delta_{x_i})$.
	
	The mapping $\psi:\X\rightarrow \R^P$ defined as 
	\begin{equation*}
	\psi(x'):=\frac{\sum_{x\in\X} \psi_{x}(x') y_{x_i}}{\sum_{x\in\X} \psi_{x}(x')}
	\end{equation*}
	belongs to $C^P(\X,\R^P)$ since it is locally a finite sum of $C^m$ functions (this also justifies the definition of $\psi$ since only a finite number of indexes are active). For any given $x'\in\X$, $\psi_{x}(x')>0$ implies that $x'\in V_i\subset \BB(x_i,\delta_{x_i})$. Hence, by definition of $ y_{x_i}$, $ y_{x_i} \in \b F(x')+\epsilon \dBB$. Since $\b F$ is convex-valued, the convex combination which defines $\psi$ leads to $\psi(x')\in \b F(x')+\epsilon \dBB$, so $\psi(\cdot)$ is the  approximate selection of class $C^m$ that we sought for.
	
	\subsection{Attempt at mimicking the proof of Rudi 2020}
	
	We look at a single affine/convex constraint $\psi$ and try to mimic the results of \citet[][Theorem 5]{rudi2020finding}. We consider the original constrained problem in the RKHS which we try approximate with kernel SOS. Assuming that the solution with constraints $\psi(x,f^*(x))\ge 0$ corresponds to an SDP operator $A^*$ such that $\psi(x,f^*(x))=\scalh{\phi(x)}{A^* \phi(x)}$,
	\begin{argminie}|s|
		{\substack{\b f \in \hh,\\ A \in S^+(\hh)}}{\underbrace{\sum_{n\in[N]} l(x_n,\b f(x_n)) + \la \|\b f\|_\hh^2}_{\Lcal(f)} + \latr \tr(A)}{\label{opt-consA}}{(\b f^*,A^*) =}%
		\addConstraint{\psi(x,f(x))}{= \scalh{\phi(x)}{A \phi(x)},\, \forall\, x\in\X\label{eq:consA_F}}
	\end{argminie}
	The approximate problem with discretization writes as follows
	\begin{argminie}|s|
		{\substack{\b f \in \hh,\\ B \in S^+(R^M)}}{\Lcal(f) + \latr \tr(B)}{\label{opt-consB}}{(\hat{\b f},\hat{B}) =}%
		\addConstraint{\psi(\tilde{x}_{m},f(\tilde{x}_{m}))}{= \scalidx{\phi_m}{B \phi_m}{\R^M},\, \forall\, m\in [M], \, \forall \, i\in [I]\label{eq:consB_F}}
	\end{argminie}
	Using \citet[][Lemma 3]{rudi2020finding}, one can show there exists $\bar B\in S^+(R^M)$ such that, for all $m$, $\scalidx{\phi_m}{\bar B \phi_m}{\R^M}=\scalh{\phi(\tilde{x}_{m})}{A \phi(\tilde{x}_{m})}$ with $\tr(\bar B)\le \tr(A^*)$. So $(f^*,\bar B)$ is admissible for \eqref{opt-consB}, hence
	\begin{equation} \label{eq:lowerbound_obj}
	\Lcal(\hat{\b f}) + \latr \tr(\hat B) \le \Lcal(f^*) + \latr \tr(\bar B)\le \Lcal(f^*) + \latr \tr(A^*)
	\end{equation}
	This gives a result similar to \citet[][Theorem 5, Step 1]{rudi2020finding}. However since the objective $\Lcal(f)$ does not appear in the constraints, we cannot merely copy \citet[][Theorem 5, Step 3]{rudi2020finding}. To have an upperbound, one would need to find a $(\hat{\b f}+f_\epsilon, \hat A_\epsilon)$ admissible for \eqref{opt-consA}, in which case, if $\Lcal$ is for instance $\beta$-Lipschitz,
	\begin{equation} \label{eq:upperbound_obj}
	\Lcal(f^*) + \latr \tr(A^*)\le \Lcal(\hat{\b f}+f_\epsilon) + \latr \tr(\hat A_\epsilon) \le \Lcal(\hat{\b f}) + \beta \|f_\epsilon\|_\hh + \latr \tr(\hat B)+err(\epsilon).
	\end{equation}
	Combining \eqref{eq:lowerbound_obj} and \eqref{eq:upperbound_obj}, one could bound $\Lcal(f^*)-\Lcal(\hat{\b f})$, but this requires to be able to construct a function $f_\epsilon\in \hh$, such that $\|f_\epsilon\|_\hh$ is small, and $\psi(x,\hat f(x)+f_\epsilon(x))\ge 0$ for all $x\in\Omega$.
	
	\citet[][Theorem 4]{rudi2020finding} gives a negative lower bound on $\psi(x,\hat f(x))$, which actually depends on $|x\mapsto\psi(x,\hat f(x))|_{\Omega,m}$, so on $\hat f$ itself. Then one would still have to build a $f_\epsilon$ as described above and ensure that $\tr(\hat A_\epsilon)$, for $\hat A_\epsilon$ corresponding to $\psi(x,f(x)+f_\epsilon(x))=\scalh{\phi(x)}{\hat A_\epsilon \phi(x)}$, is not too far from $\tr(\hat B)$.
	
	\vspace{2 cm}

	\begin{center}
		Is this the right way of considering the problem?
	\end{center}
